# Supplementary material for: Tunable and Enhanced Rashba Spin-Orbit Coupling in Iridate-Manganite Heterostructures
Source: arXiv:2004.00800 source file (2020-04-02)
Supplement: Supplementary file 1 [file Supplemental_material.pdf]

**Supplemental Material**

# Tunable and Enhanced Rashba Spin-Orbit Coupling in Iridate-Manganite Heterostructures

Thyagarajan Sumaraj Suraj[1,2 #], Ganesh Ji Omar[3,4 #], Hariom Jani [4,6], Muhammad Mangattuchali Juvaid[1,3,4], Sonu Hooda[4], Anindita Chaudhuri[5], Andrivo Rusydi[3,5], Kanikrishnan Sethupathi[2], Thirumalai Venkatesan[3,4,6,7,8], Ariando Ariando[3,4,6*], Mamidanna Sri Ramachandra Rao[1*]

[1]*Department of Physics, Nano Functional Materials Technology Center - Material Science Research Center, IIT Madras, India-600036.*

[2]*Low Temperature Physics Lab, IIT Madras, India-600036*

[3]*Department of Physics, National University of Singapore, Singapore 117542, Singapore*

[4]*NUSNNI-NanoCore, National University of Singapore, Singapore 117411, Singapore*

[5]*Singapore Synchrotron Light Source, National University of Singapore, 5 Research Link, Singapore 117603, Singapore*

[6]*National University of Singapore Graduate School for Integrative Sciences and Engineering (NGS), University Hall, 21 Lower Kent Ridge Road, Singapore 119077*

[7]*Department of Materials Science and Engineering, National University of Singapore, Singapore 117575, Singapore*

[8]*Department of Electrical and Computer Engineering, National University of Singapore, Singapore 117576, Singapore*

*corresponding authors email: ariando@nus.edu.sg , msrrao@iitm.ac.in

**Experimental Details**

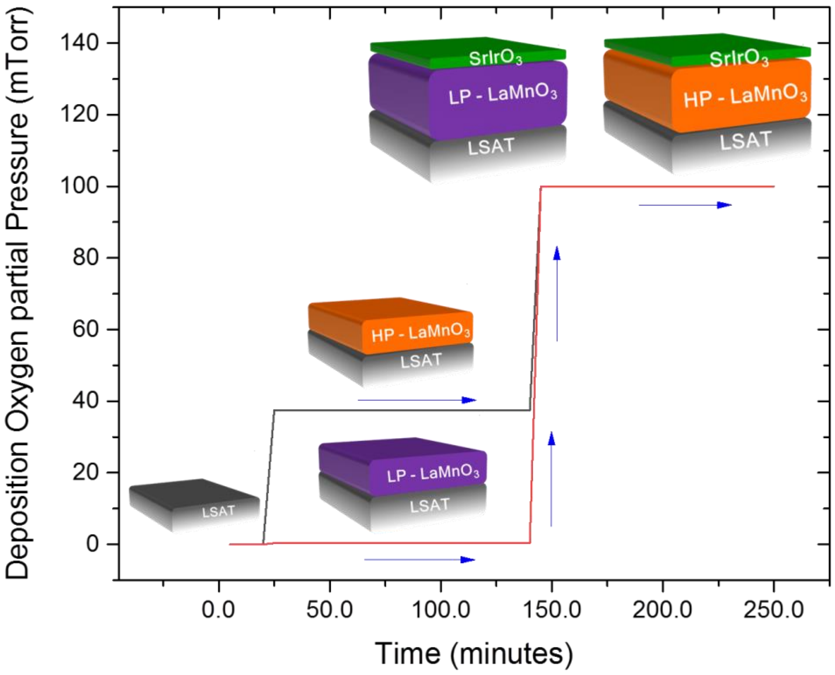


**Figure. S1**. The method adopted for LP-LMO, LP-LMO-SIO, HP-LMO and HP-LMO-SIO sample preparation with deposition $pO_2$ v/s time. Arrows are guide to the eye to point the direction of the deposition process.

Bilayers of $SrIrO_3$ on top of $LaMnO_3$ were grown on LSAT substrates along (001) orientation using pulsed laser deposition (PLD). During $LaMnO_3$ growth the chamber was evacuated to vacuum (37.5 x $10^{-3}$mTorr) to ensure $LaMnO_3$ remains in the antiferromagnetic insulating state, the oxygen excess in $LaMnO_3$ results in the formation of $Mn^{4+}$ which favours ferromagnetism through the double exchange mechanism[1-4] (this set of samples are addressed as LP-LMO-SIO samples in the rest of the manuscript). Another batch of samples was grown with 37.5 mTorr oxygen partial pressure to ensure an increase in the oxygen content in the films to transform $LaMnO_3$ into the ferromagnetic state (this set of samples will be addressed as HP-LMO-SIO samples in the rest of the manuscript). A detailed schematic with deposition pressure and time is given in **Fig. S1a**. $SrIrO_3$ was deposited at 100 mTorr $O_2$ partial pressure, then high purity oxygen was flushed into the chamber with 100 Torr $O_2$ partial pressure to eliminate oxygen

vacancies in $SrIrO_3$. Substrate temperatures were maintained at 700°C for both layers. During growth, laser parameters were kept at 1.5 J/cm$^2$ and repetition rate at 2Hz. The surface morphology of $LaMnO_3$ samples were acquired using a Park atomic force microscope (AFM). **Fig.S2 (a) and (b)** shows AFM images acquired under tapping mode. Structural measurements were carried out in a Rigaku smart lab X-ray diffractometer. XRD of $LaMnO_3$ thin films grown under LP and HP conditions with 50 nm thickness is shown in Fig.S3 (a) and (b) respectively.

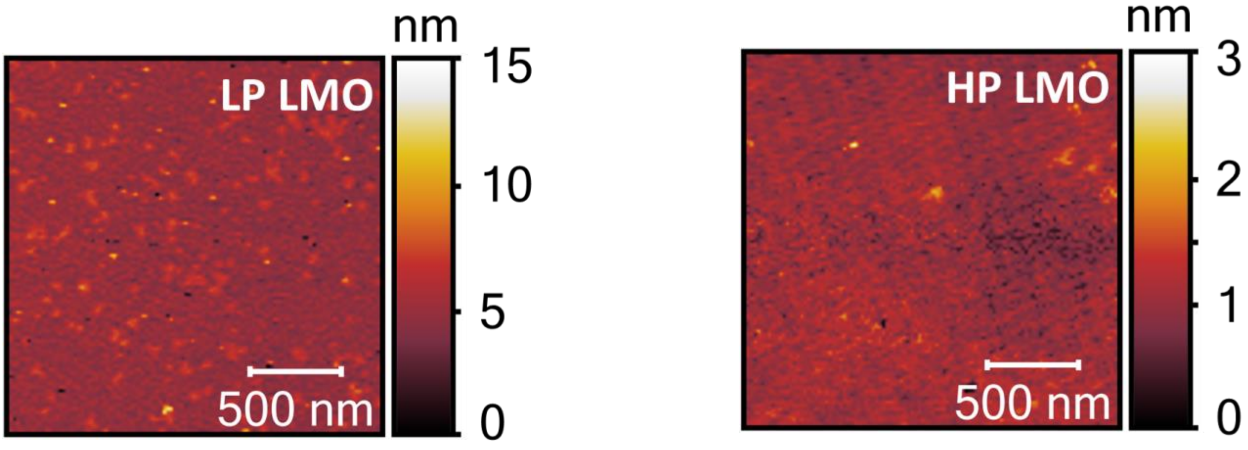


**Figure. S2**. (a) and (b) Atomic force microscopy images of LP- and HP-LMO samples respectively.

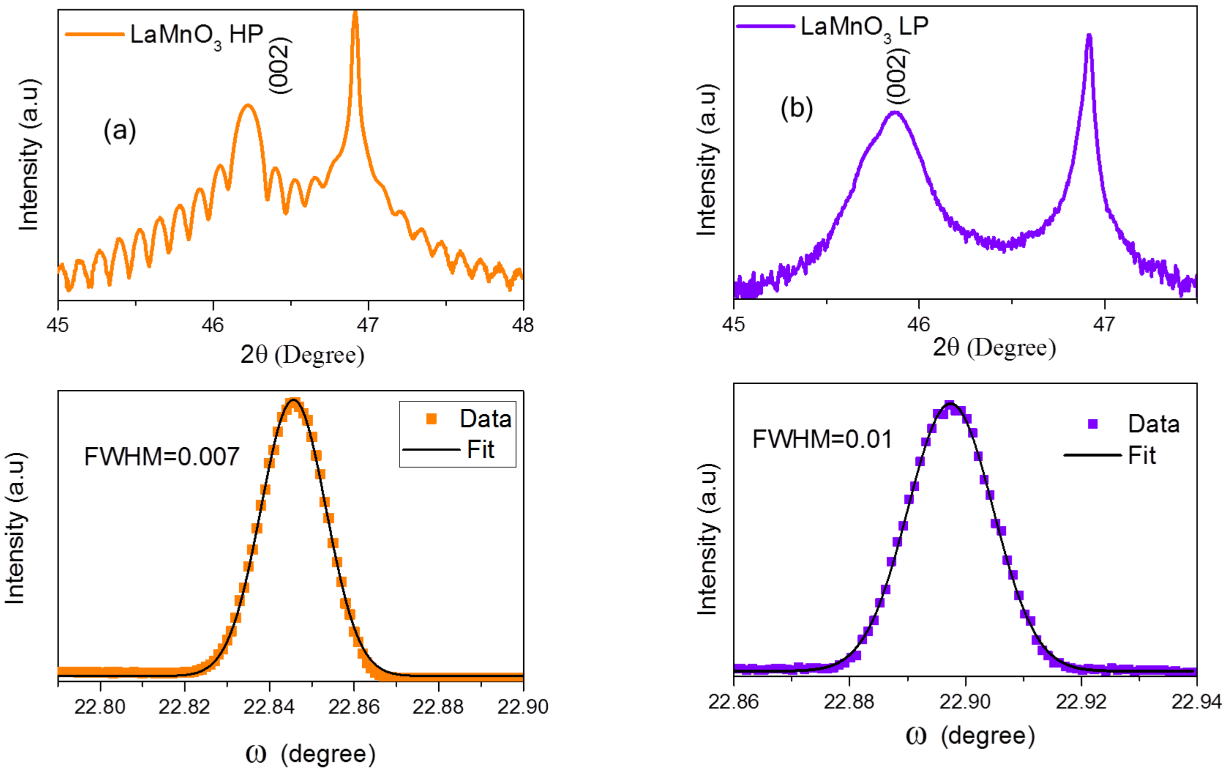


**Figure. S3**. (a) and (b) HRXRD of HP and LP LMO samples with corresponding (002) $LaMnO_3$ peak rocking curve scan in the inset. Also, the inset shows AFM images taken on LP and HP samples and their RMS roughness respectively.

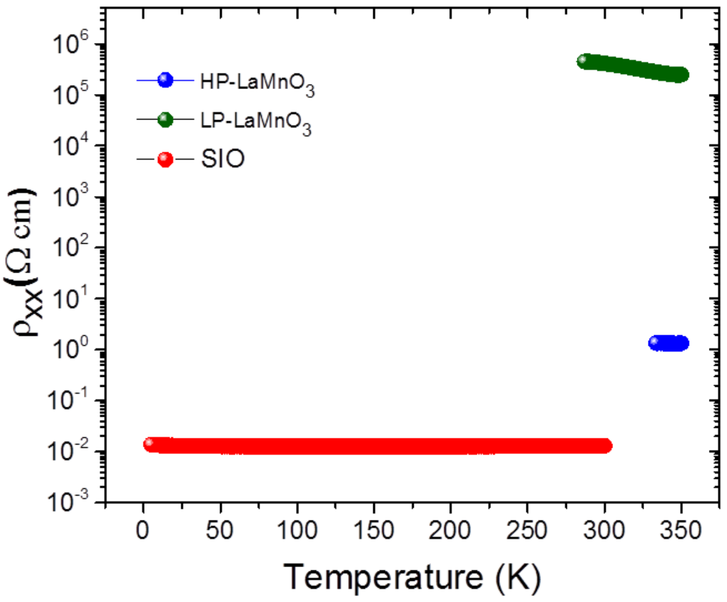


**Figure. S4**. Resistivity of the $LaMnO_3$ deposited at $37.5\times10^{-3}$ Torr and deposited at 37.5 mTorr also $SrIrO_3$ samples directly grown on LSAT(001) substrate.

For electrical characterization, Hall bar devices were patterned using photolithography and the channel sizes were 50µm X 150µm. An insulating AlN layer was used for masking the device from the rest of the device area, on LSAT substrates prior to oxide layer deposition. For electrical measurements, Quantum Design PPMS with a high resolution horizontal rotating holder was used. All electrical contacts were bonded with Aluminum wires using a wire bonder. All electrical measurements were performed simultaneously on control $LaMnO_3$ samples grown at the same conditions mentioned earlier and have also been annealed at 100 mTorr ($SrIrO_3$ growth pressure). Transport measurements revealed that these control samples are more insulating by at least three orders in magnitude more (shown in Fig: S6). Similarly, control $SrIrO_3$ samples were also grown for on LSAT at 100 mTorr $O_2$ partial pressure for transport characterization. Magnetic measurements were carried out in MPMS XL SQUID based vibrating sample magnetometer. XAS measurements were taken in Singapore Synchrotron light Source (SSLS) in TEY mode.

To determine the Mn valence states XPS was carried out using the SPECS XPS system with a PHOIBOS-100 energy analyzer, using Aluminium (Kα: 1486.61 eV) X-ray source. The surface of HP-LMO and LP-LMO were etched in-situ using Ar ion beams before scanning to avoid surface contaminations in the spectra.$Mn^{3+}$ and $Mn^{4+}$ peaks were deconvoluted from the Mn $2p_{3/2}$ spectra. The ratio of $Mn^{4+}$ to $Mn^{3+}$ was deduced from the area under the curve and found to be 0.98 for HP-LMO and 0.35 for LP-LMO.

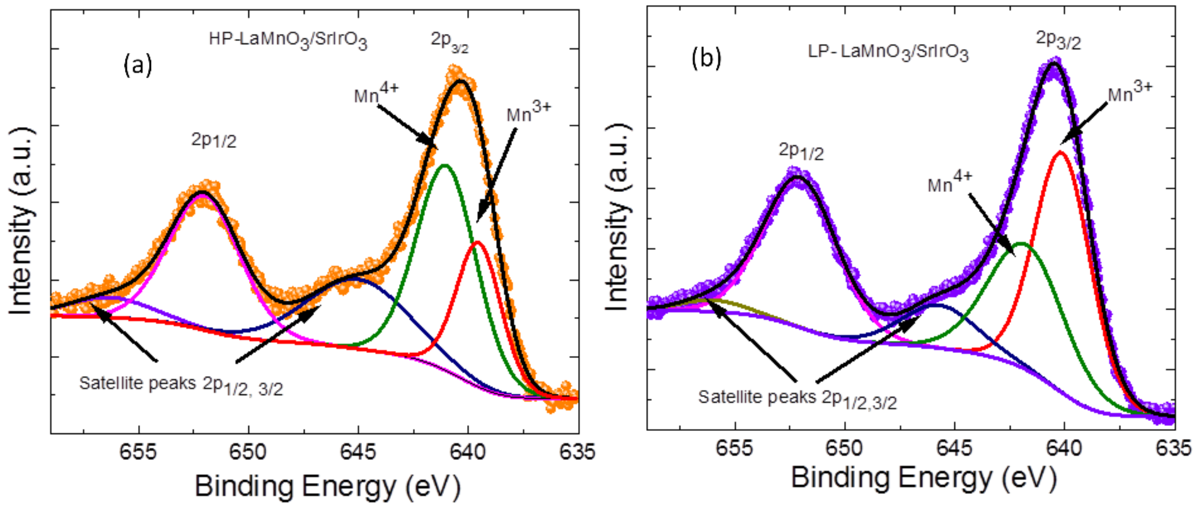


**Figure .S5**. (a) and (b) The X-ray photoelectron spectroscopy performed on HP- and LP-LMO-SIO samples with $SrIrO_3$ being etched with Ar ion milling in the XPS chamber in-situ. The deconvoluted peaks show the respective Mn valence states present in the system.

Rutherford Backscattering Spectrometry (RBS) was carried out using 3.5 MV Singletron Accelerator at CIBA, NUS. A 2 MeV $He^+$ beam was used for film thickness and stoichiometry analysis. The films were grown on lighter substrate MgO instead of LSAT (following similar growth conditions), for a clear signal from the film in RBS measurements. Typical RBS spectrum fitted using simulation code SIMNRA is shown in figure S6 (a). The La/Mn ratio and oxygen content were analyzed by fitting the RBS data. Figure S6 (b,c) shows the La/Mn ratio and oxygen content in LMO films, as a function of deposition oxygen partial pressure.

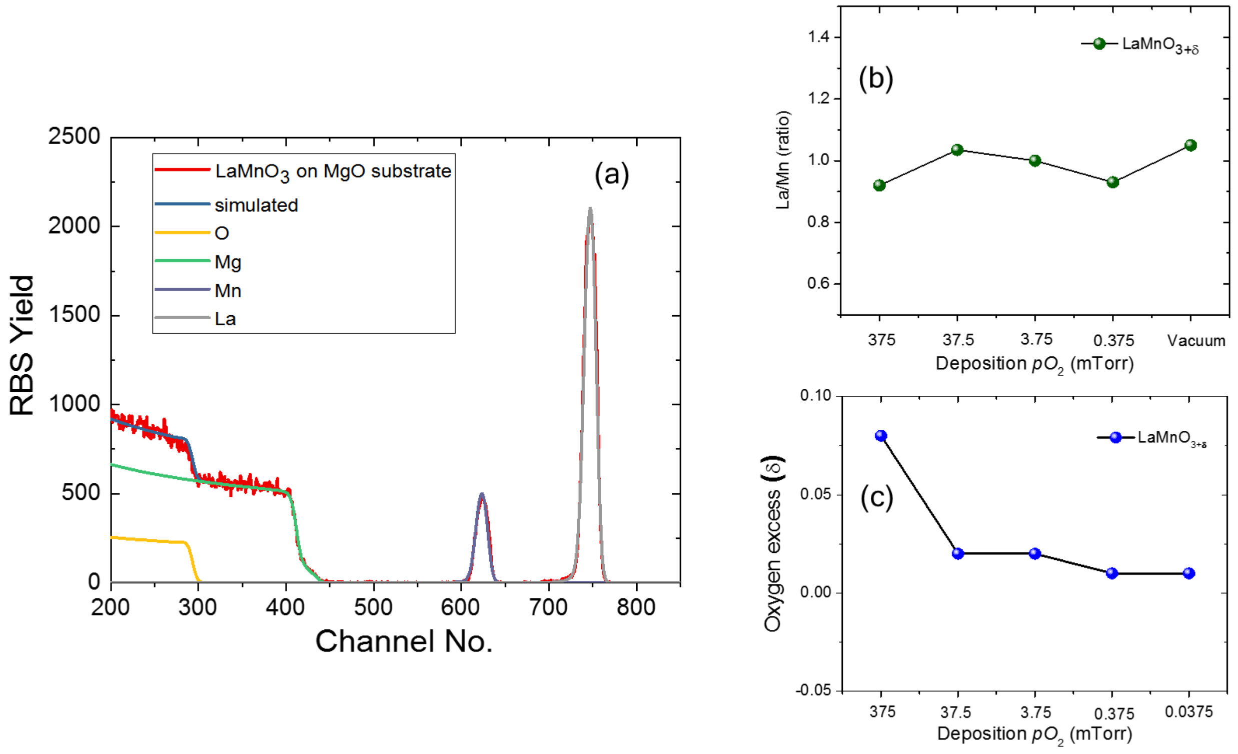


**Figure. S6**. (a) The RBS spectra taken on $LaMnO_3$ thin films deposited on MgO substrates (LSAT is heavier compared to $LaMnO_3$) , MgO substrate will show clean spectra with less background. (b) La/Mn ratio has also been estimated as a function of deposition oxygen partial pressure. (c) The rough estimate of oxygen content in the $LaMnO_3$ thin films as a function of oxygen partial pressure.

## References


1 J. Töpfer and J. B. Goodenough, Journal of Solid State Chemistry **130**, 117 (1997).

2 Q. Huang, A. Santoro, J. W. Lynn, R. W. Erwin, J. A. Borchers, J. L. Peng, and R. L. Greene, Physical Review B **55**, 14987 (1997).

3 C. Ritter, M. R. Ibarra, J. M. De Teresa, P. A. Algarabel, C. Marquina, J. Blasco, J. García, S. Oseroff, and S. W. Cheong, Physical Review B **56**, 8902 (1997).

4 J. Roqueta, et al., Crystal Growth & Design **15**, 5332 (2015).
